# Supplementary material for: Structure and dynamics in yttrium-based molten rare earth alkali fluorides
Source: arXiv:1302.4563 source file (2013-05-13)
Supplement: Supplementary file 1 [file si.pdf]

# Supplementary Material for "Structure and dynamics in yttrium-based molten rare earth alkali fluorides"

Maximilien Levesque,[1, a)] Vincent Sarou-Kanian,[2, 3] Mathieu Salanne,[4, b)] Mallory Gobet,[2, 3, 5] Henri Groult,[4] Catherine Bessada,[2, 3] Paul A. Madden,[1] and Anne-Laure Rollet[4]
[1)] *Department of Materials, University of Oxford, Parks Road, Oxford OX1 3PH, United Kingdom*
[2)] *CNRS, UPR3079, CEMHTI, 1D avenue de la Recherche Scientifique, 45071 Orléans cedex 2, France*
[3)] *Faculté des sciences, Université d'Orléans, avenue du Parc Floral, BP 6749, 45067 Orléans cedex 2, France*
[4)] *UPMC Univ Paris 06, CNRS, ESPCI, UMR 7195, PECSA, F-75005, Paris, France*
[5)] *Hunter College of the City University of New York, Department of Physics & Astronomy, New York, NY 10065, USA*

## I. MOLECULAR DYNAMICS POLARIZABLE FORCE FIELD

The charge-charge term is naturally

$$V^{\mathrm{qq}}\left(r_{ij}\right)=\sum_{i,j>i}\frac{q_iq_j}{r_{ij}},\qquad(1)$$

where $q_i$ is the formal charge on ion $i$ and $r_{ij}$ is the distance between ions $i$ and $j$. The dispersion component captures dipole-dipole and dipole-quadrupole terms. It reads

$$V^{\mathrm{disp}}\left(r_{ij}\right)=-\sum_{i,j>i}\left[f_6^{ij}\left(r_{ij}\right)\frac{C_6^{ij}}{r_{ij}^6}+f_8^{ij}\left(r_{ij}\right)\frac{C_8^{ij}}{r_{ij}^8}\right],\qquad(2)$$

where $C_6^{ij}$ ($C_8^{ij}$) is the dipole-dipole (dipole-quadrupole) dispersion coefficient, and $f_{6,8}^{ij}$ are Tang-Toennies dispersion damping functions[1]. They describe the short range correction to the asymptotic multipole expansion of dispersion[2]. They are expressed as

$$f_n^{ij}\left(r_{ij}\right)=1-c_n^{ij}\exp\left(-b_n^{ij}r_{ij}\right)\sum_{k=0}^{n}\frac{\left(b_n^{ij}r_{ij}\right)^k}{k!},\qquad(3)$$

where $b_n^{ij}$ is the distance at which the correction starts to be taken into account, and $c_n^{ij}=1$, ensuring that the dispersion term is cancelled for short distances. The repulsion overlap component is given by

$$V^{\mathrm{rep}}\left(r_{ij}\right)=\sum_{i,j>i}A^{ij}\exp\left(-a^{ij}r_{ij}\right),\qquad(4)$$

where $A^{ij}$ and $a^{ij}$ are also parameters deduced from first principles. Finally, the interatomic potential includes charge-dipole and dipole-dipole polarizations:

$$V^{\mathrm{pol}}\left(r_{ij}\right)=\sum_{i,j>i}\left(q_i\mu_{j,\alpha}f_4^{ij}\left(r_{ij}\right)-q_j\mu_{i,\alpha}f_4^{ji}\left(r_{ij}\right)t\right)T_\alpha^{(1)}-\sum_{i,j>i}\mu_{i,\alpha}\mu_{j,\beta}T_{\alpha,\beta}^{(2)}\left(\mathbf{r}_{ij}\right)+\sum_i\frac{1}{2\alpha_i}\mu_i^2.\qquad(5)$$

Here, $T_\alpha^{(1)}$ and $T_{\alpha,\beta}^{(2)}$ are the charge-dipole and dipole-dipole interaction tensors, and $\alpha_i$ is the polarization of ion $i$. Tang-Toennies functions are again included to account for the short-range effects. The induced dipoles $\mu_i$ are three-dimensional vectors. At each time step, they are relaxed adiabatically and self-consistently in order to minimize $V^{\mathrm{pol}}$. The inter atomic potential parameters are given in reference[3].

## II. CONDITIONS OF THE MOLECULAR DYNAMICS SIMULATIONS

The setups of the molecular dynamics simulations are summarized in table I. The simulation cell is cubic.

| $x_{\mathrm{YF_3}}$ (mol. %) | $N_{\mathrm{tot}}$ | $N_{\mathrm{F}}$ | $N_{\mathrm{Y}}$ | $N_{\mathrm{Li}}$ | $L$ (Å) |
|---|---|---|---|---|---|
| 10.00 | 550 | 300 | 25 | 225 | 19.09 |
| 15.22 | 530 | 300 | 35 | 195 | 18.95 |
| 20.09 | 514 | 300 | 43 | 171 | 18.83 |
| 25.00 | 500 | 300 | 50 | 150 | 18.72 |
| 29.79 | 488 | 300 | 56 | 132 | 18.63 |
| 35.23 | 476 | 300 | 62 | 114 | 18.54 |
| 40.36 | 466 | 300 | 67 | 99 | 18.48 |
| 44.94 | 458 | 300 | 71 | 87 | 18.41 |
| 50.00 | 450 | 300 | 75 | 75 | 18.34 |
| 55.63 | 442 | 300 | 79 | 63 | 18.28 |
| 60.29 | 436 | 300 | 82 | 54 | 18.26 |

TABLE I. Conditions of the molecular dynamics simulations, where $x_{\mathrm{YF_3}}$ is the molecular fraction of $YF_3$, $N_{\mathrm{tot}}$ is the total number of atoms in the simulation supercell, $N_\alpha$ is the total number of atoms of type $\alpha$, and $L$ is the length of the cell.

[a)] Electronic mail: maximilien.levesque@gmail.com
[b)] Electronic mail: mathieu.salanne@upmc.fr

## III. ELECTRICAL CONDUCTIVITY POTENTIOMETRIC MEASUREMENTS

A scheme of the setup used to measure the electrical conductivity of molten LiF-$YF_3$ salts is given in figure 1.

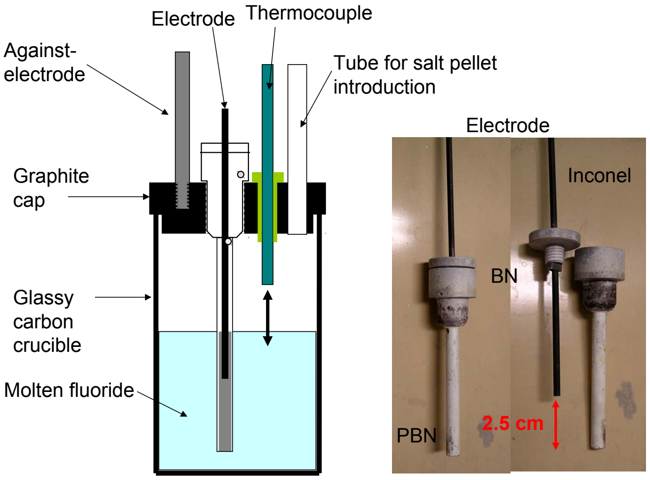


FIG. 1. Experimental setup for the electrical conductivity potentiometric measurements.

[1] K. T. Tang and J. P. Toennies, J. Chem. Phys. **80**, 3726 (1984).
[2] A. J. Stone, *Theory of intermolecular forces* (Oxford University Press, Oxford, 1996).
[3] M. Salanne, B. Rotenberg, C. Simon, S. Jahn, R. Vuilleumier, and P. A. Madden, Theor. Chem. Acc. **131**, 1143 (2012).
